# Supplementary material for: Explaining Chest X-ray Pathologies in Natural Language
Source: arXiv:2207.04343 source file (2022-07-09)
Supplement: Supplementary file 1 [file mimic-nle.tex]

\section{Processing Steps to generate MIMIC-NLE}

This section contains additional details on the processing steps required to create the MIMIC-NLE dataset. 

Our NLEs form a subset of the MIMIC-CXR database, which contains 227,835 radiographic studies performed at the Beth Israel Deaconess Medical Center in Boston, MA \cite{johnsonMIMICCXRJPGLargePublicly2019a}. We only consider PA or AP scans, as lateral scans as they are taken less frequently in practice and most studies have either of the frontal scans.

The first step in extracting NLEs is to extract the finding and impression section, which contain the descriptive part of a scan, using an NLP tool provided by the MIMIC-CXR authors \footnote{\url{https://github.com/MIT-LCP/mimic-cxr}}. Out of the total of 227,835 reports, 10,590 contain neither a findings nor an impression section and are therefore skipped. From the other reports, we then extract individual sentences using the spacy sentencizer. We get a total of 1,383,533 sentences. 

For each of these sentences we then tag explanation keyword and extract the labels referred to in the sentence. We tag the following set of keywords (case insensitive): ``indicate'', ``suggest'', ``concerning for'', ``compatible with'', ``account'', ``due'', ``reflect'', ``relate'', ``potentially'', ``likely represent'', ``suspicious for'', ``worrisome for'', ``consistent with'', ``may represent''. We add the exemptions ``suggestion'', ``is suggested'', ``correlate'' to leave out some corner cases. This selection is based on in-house knowledge, empirical evidence, and a survey of radiologists conducted in \cite{mityul_interpretive_2018}. In order to extract labels referred to in a sentence, we use the pre-trained CheXbert model from \cite{smit_combining_2020}. ChexBert extracts the following 14 labels from free-text: 'Enlarged Cardiomediastinum', 'Cardiomegaly', 'Lung Opacity', 'Lung Lesion', 'Edema', 'Consolidation', 'Pneumonia', 'Atelectasis', 'Pneumothorax', 'Pleural Effusion', 'Pleural Other', 'Fracture', 'Support Devices', 'No Finding'. These correspond to the labels extracted for the CheXpert \cite{irvin_chexpert_2019} dataset and were chosen for their frequency and clinical relevance in chest X-rays. We use the implementation and pre-trained weights from their Github repository \footnote{\url{https://github.com/stanfordmlgroup/CheXbert}}. For each label, CheXbert predicts whether it's ``Positive'', ``Uncertain'', ``Negative'', or not mentioned. We only extract labels for which the uncertainty label is ``Positive'' or ``Uncertain''.

One of the advantages of clinical reports is that they use relatively structured language and therefore this small set of keywords covers the major part of all explanations. However, upon inspecting the extracted sentences we notice that some explanation keywords, such as ``due'', are also used to explain factors unrelated to a uncertain or positive viewpoint, such as issues caused by the patient positioning (e.g., ``Assessment is somewhat limited due to patient positioning and exclusion of the left costophrenic angle.''). We devise three categories of keywords that indicate that a sentence is not an NLE solely based on findings made in the scan. They include sentences that explain things based on patient history (``prior'', ``compare'', ``change'', ``deteriorat'', ``increase'', ``decrease'', ``previous'', ``patient''), recommendations for follow-up procedures which use many of the same keywords (``recommend'', ``perform'', ``follow''), keywords about technical aspects of the procedure, such as patient positioning (``CT'', ``technique'', `` position'', ``exam'', ``assess'', ``view'', ``imag''), and lastly also the keyword ``finding'', as it is often used to explain a diagnosis without us knowing which findings are meant. After removing 79,068 sentences containing anonymized data (containing an underscore ``\_'' somewhere), a further 297,463 sentences are removed based on the keywords.

Based on tagged explanation keywords and extracted labels from each sentence, and the rules outlined in Table \ref{tab:lbl_rules}, we are then able to extract 43,612 NLEs from the remaining sentences. As a final step, we remove duplicates NLEs from each report. A duplicate NLE occurs when the same labels are mentioned in a sentence belonging to the same study. This usually happens when an NLE is repeated in the impression section. This leaves us with the final dataset size of 39,094 NLEs. Afterward we only consider NLEs for studies with either AP or PA images. This removes another 1,091.

Quite frequently chexBert finds labels in an NLE that are not marked on the overall image. In fact, for 17,982 of the explanations that was the case. Manual checking showed that this was mostly due to the poor performance of chexpert compared to chexbert. Some few cases were also false positives by chexbert. 

Table XX shows
